# Supplementary material for: Calorimetric measurement of work for a driven harmonic oscillator
Source: arXiv:1607.02342 ancillary file (2016-09-16)
Supplement: Supplementary file 1 [file QHO-cal-SM.pdf]

# Supplementary Material on Calorimetric measurement of work for a driven harmonic oscillator


Rui Sampaio and Samu Suomela
*COMP Center of Excellence, Department of Applied Physics,*
*Aalto University, P.O. Box 11000, FI-00076 Aalto, Finland*

Tapio Ala-Nissila
*COMP Center of Excellence, Department of Applied Physics,*
*Aalto University, P.O. Box 11000, FI-00076 Aalto, Finland and*
*Department of Physics, P.O. Box 1843, Brown University, Providence, Rhode Island 02912-1843, U.S.A.*


## I. COEFFICIENTS FOR MOMENTS OF WORK

For the first moment, the first three terms in Eq. (17) of the main text are given by

$$w_{01} = \frac{\mu e^{\beta\omega_0 - \mu}}{z_2}\, {}_1F_1\left(\frac{z_2}{z_1}; \frac{z_3}{z_1}; \mu\right); \tag{1}$$

$$w_{11} = \frac{\mu e^{\beta\omega_0 - \mu}}{z_2^2}\left(\mu\, {}_1F_1\left(\frac{z_2}{z_1}; \frac{z_3}{z_1}; \mu\right) - z_2\, {}_1F_1\left(\frac{1}{z_1}; \frac{z_2}{z_1}; \mu\right) - \frac{2(\mu-1)z_2}{z_3}\, {}_1F_1\left(\frac{z_3}{z_1}; \frac{z_4}{z_1}; \mu\right) + \frac{\mu z_2}{z_4}\, {}_1F_1\left(\frac{z_4}{z_1}; \frac{z_5}{z_1}; \mu\right)\right); \tag{2}$$

$$\begin{aligned} w_{21} = &\frac{\mu e^{\beta\omega_0 - \mu}}{2 z_2 z_3}\left[\frac{z_2\mu^2}{z_6}\, {}_1F_1\left(\frac{z_6}{z_1}; \frac{z_7}{z_1}; \mu\right) + \frac{z_2 6(\mu-1)^2}{z_4}\, {}_1F_1\left(\frac{z_4}{z_1}; \frac{z_5}{z_1}; \mu\right) - \frac{4 z_2 \mu(\mu-1)}{z_3}\, {}_1F_1\left(\frac{z_3}{z_1}; \frac{z_4}{z_1}; \mu\right)\right. \\ &\left. + \frac{2\mu z_2(3-2\mu)}{z_5}\, {}_1F_1\left(\frac{z_5}{z_1}; \frac{z_6}{z_1}; \mu\right) + (\mu(\mu+4)-4)\, {}_1F_1\left(\frac{z_2}{z_1}; \frac{z_3}{z_1}; \mu\right) - 2\mu z_2\, {}_1F_1\left(\frac{1}{z_1}; \frac{z_2}{z_1}; \mu\right)\right], \end{aligned} \tag{3}$$

where ${}_1F_1(a, b; \mu)$ is the Kummer confluent hypergeometric function, $z_1 = \left(1 + e^{\beta\omega_0}\right)$ and $z_i = \left(i + (i-1)e^{\beta\omega_0}\right)$ for $i > 1$. Similarly, for the second moment,

$$w_{02} = w_{01}; \tag{4}$$

$$\begin{aligned} w_{12} = &\frac{e^{\beta\omega_0 - \mu}}{z_2^2}\left[\frac{3\mu^2 z_2}{z_4}\, {}_1F_1\left(\frac{z_4}{z_1}; \frac{z_5}{z_1}; \mu\right) + \mu z_2\, {}_1F_1\left(\frac{1}{z_1}; \frac{z_2}{z_1}; \mu\right);\right. \\ &\left. - \frac{2(3\mu-5)\mu z_2}{z_3}\, {}_1F_1\left(\frac{z_3}{z_1}; \frac{z_4}{z_1}; \mu\right) + (\mu-2)(3\mu-2)\, {}_1F_1\left(\frac{z_2}{z_1}; \frac{z_3}{z_1}; \mu\right)\right] \end{aligned} \tag{5}$$

$$\begin{aligned} w_{22} = &\frac{e^{\beta\omega_0 - \mu}}{2 z_2 z_3}\left[2\mu^2 z_2\, {}_1F_1\left(\frac{1}{z_1}; \frac{z_2}{z_1}; \mu\right) + \frac{5 z_2 \mu^3}{z_6}\, {}_1F_1\left(\frac{z_6}{z_1}; \frac{z_7}{z_1}; \mu\right)\right. \\ &+ \frac{2 z_2(21-10\mu)\mu^2}{z_5}\, {}_1F_1\left(\frac{z_5}{z_1}; \frac{z_6}{z_1}; \mu\right) + \frac{6 z_2(\mu-1)(5\mu-13)\mu}{z_4}\, {}_1F_1\left(\frac{z_4}{z_1}; \frac{z_5}{z_1}; \mu\right) \\ &\left. - \frac{4 z_2(\mu-1)(\mu(5\mu-18)+6)}{z_3}\, {}_1F_1\left(\frac{z_3}{z_1}; \frac{z_4}{z_1}; \mu\right) + (\mu(5\mu-28)+28) z_2 \mu\, {}_1F_1\left(\frac{z_2}{z_1}; \frac{z_3}{z_1}; \mu\right)\right]. \end{aligned} \tag{6}$$

## II. MOMENTS OF WORK IN THE TWO MEASUREMENT PROTOCOL FOR A DRIVEN DAMPED HARMONIC OSCILLATOR

### A. Limit of unitary evolution

In the unitary limit there is no heat exchange (and therefore no jumps in the trajectory). From Eq. (6) in the main text with $Q = 0$ we can write

$$\langle W^k \rangle_{\mathrm{u}} = \sum_{n,m} p_{\mathrm{eq}}(n) p(m|n)(E_m - E_n)^k, \tag{7}$$

with $p(m|n) = \left|\langle m|\hat{U}_D(T)|n\rangle\right|^2$, where $\hat{U}_{\rm u}(T)$ is given by Eq. (16) in the main text, $p_{\rm eq}(n)$ is the thermal equilibrium distribution, the subscript $u$ indicates that the average is taken over unitary evolution, and $|n\rangle$ and $|m\rangle$ are eigenfunctions of $\hat{H}_0$ (see the main text).For the average work becomes

$$\begin{aligned}
\langle W(t)\rangle_{\rm u} &= \frac{\hbar\omega_0}{Z}\sum_n e^{-\beta\omega_0 n}\sum_m \left|\langle m|e^{-i\sqrt{2\mu(t)}\hat{P}}|n\rangle\right|^2 (m-n) \\
&= \frac{\hbar\omega_0}{Z}\sum_n e^{-\beta\omega_0 n}\sum_m \langle n|e^{+i\sqrt{2\mu(t)}\hat{P}}|m\rangle\langle m|e^{-i\sqrt{2\mu(t)}\hat{P}}|n\rangle(m-n) \\
&= \frac{\hbar\omega_0}{Z}\sum_n e^{-\beta\omega_0 n}\langle n|e^{+i\sqrt{2\mu(t)}\hat{P}}\sum_m |m\rangle(m-n)\langle m|e^{-i\sqrt{2\mu(t)}\hat{P}}|n\rangle \\
&= \frac{\hbar\omega_0}{Z}\sum_n e^{-\beta\omega_0 n}\mu(t) \\
&= \hbar\omega_0\mu(t),
\end{aligned} \tag{8}$$

and the variance

$$\begin{aligned}
\sigma^2_{W_{\rm u}}(t) = \langle W^2(t)\rangle_{\rm u} - \langle W(t)\rangle^2_{\rm u} &= \frac{(\hbar\omega_0)^2}{Z}\sum_n e^{-\beta\omega_0 n}\sum_m \left|\langle m|e^{-i\sqrt{2\mu(t)}\hat{P}}|n\rangle\right|^2 (m-n)^2 - \mu^2(t) \\
&= \frac{(\hbar\omega_0)^2}{Z}\sum_n e^{-\beta\omega_0 n}\langle n|e^{+i\sqrt{2\mu(t)}\hat{P}}\sum_m |m\rangle(m-n)^2\langle m|e^{-i\sqrt{2\mu(t)}\hat{P}}|n\rangle \\
&= \frac{(\hbar\omega_0)^2}{Z}\sum_n e^{-\beta\omega_0 n}\left(\mu(n+\frac{1}{2}) + \mu^2\right) - \mu^2(t) \\
&= 2\,(\hbar\omega_0)^2\left(N + \frac{1}{2}\right)\mu(t),
\end{aligned} \tag{9}$$

where $\mu(t) = (\lambda_0 T/2\hbar)^2$, $N \equiv [\exp(\beta\omega_0) - 1]^{-1}$ is the average thermal occupation number, and we've used the relations

$$e^{+i\sqrt{2\mu(t)}\hat{P}}\sum_m |m\rangle(m-n)\langle m|e^{-i\sqrt{2\mu(t)}\hat{P}} = e^{+i\sqrt{2\mu(t)}\hat{P}}\left(\hat{H}_0 - n\right)e^{-i\sqrt{2\mu(t)}\hat{P}} = (\hat{H}_0 - n) + x_0\hat{X} + \mu(t)\ , \tag{10}$$

$$\begin{aligned}
e^{+i\sqrt{2\mu(t)}\hat{P}}\sum_m |m\rangle(m-n)\langle m|e^{-i\sqrt{2\mu(t)}\hat{P}} &= e^{+i\sqrt{2\mu(t)}\hat{P}}\left(\hat{H}_0^2 - 2n\hat{H}_0 + n^2\right)e^{-i\sqrt{2\mu(t)}\hat{P}} \\
&= \left(\hat{H}_0 + x_0\hat{X} + \mu(t)\right)^2 - 2n\left(\hat{H}_0 + x_0\hat{X} + \mu(t)\right) + n^2.
\end{aligned} \tag{11}$$

### B. Open System evolution

In the open system evolution limit, the system cannot be approximated as closed and the dissipative term $D$ in Eq. (5) in the main text must be included, together with stochastic trajectories with jumps. The main quantity to be evaluated is transmission coefficient encoding the probability for a particular trajectory with $N$ jumps, $T_N(m,t;i_N,t_N;\ldots;i_1,t_1|n)$, given by equation (11) in the main text. Using the relations

$$\hat{C}_0\hat{U}_{\rm nh}(t) = \gamma_0^{1/2}\hat{U}_{\rm nh}(t)\left[e^{-\frac{\gamma_\Sigma}{2}t}\hat{a} + \frac{\lambda_0}{\hbar\gamma_\Sigma}\left(e^{-\frac{\gamma_\Sigma}{2}t} - 1\right)\right] = \hat{U}_{\rm nh}(t)\hat{C}'_0(t); \tag{12}$$

$$\hat{C}_1\hat{U}_{\rm nh}(t) = \gamma_1^{1/2}\hat{U}_{\rm nh}(t)\left[e^{\frac{\gamma_\Sigma}{2}t}\hat{a}^\dagger + \frac{\lambda_0}{\hbar\gamma_\Sigma}\left(e^{\frac{\gamma_\Sigma}{2}t} - 1\right)\right] = \hat{U}_{\rm nh}(t)\hat{C}'_1(t), \tag{13}$$

where $\hat{C}'_i(t) = a_i(t)\hat{C}_i + \gamma_i^{1/2}b_i(t)$ with $a_i(t) = e^{-(-1)^i\gamma_\Sigma t/2}$ and $b_i(t) = \lambda_0/(\hbar\gamma_\Sigma)[a_i(t) - 1]$, we can write

$$T_N(m,t;i_N,t_N;\ldots;i_1,t_1|n) = \left|\langle m|\hat{U}_{\rm nh}(T)\hat{C}'_{i_N}(t_N)\ldots\hat{C}'_{i_1}(t_1)|n\rangle\right|^2. \tag{14}$$

It remains to evaluate $u(m,t|n) \equiv \langle m|\hat{U}_{\rm nh}(T)|n\rangle$ for arbitrary $n$. To this end we employ second order perturbation theory to expand $\hat{U}_{\rm nh}(T)$ as

$$\hat{U}_{nh} \approx e^{-\frac{i}{\hbar}\frac{\lambda_0 t}{\sqrt{2}}\hat{P}}\left(1-\frac{i}{\hbar}\int_0^t \mathrm{d}t_1\hat{D}(t_1)-\frac{1}{\hbar^2}\int_0^t \mathrm{d}t_1\int_0^{t_1}\mathrm{d}t_2\hat{D}(t_1)\hat{D}(t_2)\right)\,, \tag{15}$$

where

$$\begin{aligned}\hat{D}(t) \equiv& \exp(\frac{i}{\hbar}\frac{\lambda_0 t}{\sqrt{2}}\hat{P})\hat{D}\exp(-\frac{i}{\hbar}\frac{\lambda_0 t}{\sqrt{2}}\hat{P})\\ =&-i\frac{\gamma_\Sigma}{2}\left(\hat{a}^\dagger\hat{a}+\frac{\gamma_\uparrow}{\gamma_\Sigma}+\mu(t)+\sqrt{2\mu(t)}\hat{X}\right)\\ =&-i\frac{\gamma_\Sigma}{2}\left(\hat{H}'(t)+\sqrt{2\mu(t)}\hat{X}\right),\end{aligned} \tag{16}$$

and $\hat{H}'(t)=\hat{a}^\dagger\hat{a}+\gamma_\uparrow/\gamma_\Sigma+\mu(t)$ is diagonal in the energy eigenbasis. Carrying out the time integration in Eq. (15) yields

$$u(m,t|n)=U_0^{mn}(t)+\frac{\gamma_\Sigma}{2}U_1^{mn}(t)+\frac{\gamma_\Sigma^2}{4}U_2^{mn}(t), \tag{17}$$

with

$$U_0^{mn}(t)=I^0_{mn}(t); \tag{18}$$

$$U_1^{mn}(t)=-\left(nt+\frac{\gamma_\uparrow}{\gamma_\Sigma}t+\frac{\lambda_0^2}{12}t^3\right)I^0_{mn}(t)-\frac{\lambda_0}{2\sqrt{2}}t^2 I^1_{mn}(t); \tag{19}$$

$$\begin{aligned}U_2^{mn}(t)=&\left[\frac{t^2\left(12\gamma_\uparrow+12\gamma_\Sigma n+\gamma_\Sigma\lambda_0^2t^2\right)^2}{288\gamma_\Sigma^2}I^0_{mn}(t)+\frac{\lambda_0 t^3\left(20\gamma_\Sigma+20\gamma_\uparrow n+\gamma_\Sigma\lambda_0^2t^2\right)}{60\sqrt{2}\gamma_\Sigma}I^1_{mn}(t)\right.\\ &+\frac{\lambda_0\sqrt{n+1}t^3\left(20(\gamma_\Sigma+\gamma_\uparrow+\gamma_\Sigma n)+3\gamma_\Sigma\lambda_0^2t^2\right)}{240\gamma_\Sigma}I^0_{m(n+1)}(t)\\ &+\frac{\lambda_0\sqrt{n}t^3\left(20(\gamma_\uparrow+\gamma_\Sigma(n-1))+3\gamma_\Sigma\lambda_0^2t^2\right)}{240\gamma_\Sigma}I^0_{m(n-1)}(t)\\ &\left.+\frac{\lambda_0^2}{16}t^4I^2_{mn}(t)\right],\end{aligned} \tag{20}$$

with

$$I^0_{mn}(t)=\frac{e^{-x_0^2/4}}{\sqrt{2^{m+n}n!m!}}\sum_{k=0}^m\binom{m}{k}\binom{n}{k}2^k k!(-1)^{n-k}x_0^{m+n-2k}; \tag{21}$$

$$\begin{aligned}I^1_{mn}(t)=&-\frac{x_0}{2}I^0_{mn}(t)\\ &+\frac{e^{-x_0^2/4}}{\sqrt{2^{m+n}n!m!}}\sum_{k=0}^m\sum_{l=0}^n\binom{m}{k}\binom{n}{l}(-1)^{n-l}\sqrt{2^{k+l}k!l!}x_0^{m+n-k-l}\begin{cases}\sqrt{\frac{l+1}{2}} & \text{, if } k=l+1;\\ \sqrt{\frac{l}{2}} & \text{, if } k=l-1;\\ 0 & \text{, otherwise;}\end{cases}\end{aligned} \tag{22}$$

$$\begin{aligned}I^2_{mn}(t)=&-\frac{x_0^2}{4}I^0_{mn}(t)-x_0I^1_{mn}(t)\\ &+\frac{e^{-x_0^2/4}}{\sqrt{2^{m+n}n!m!}}\sum_{k=0}^m\sum_{l=0}^n\binom{m}{k}\binom{n}{l}(-1)^{n-l}\sqrt{2^{k+l}k!l!}x_0^{m+n-k-l}\begin{cases}\frac{1}{2}\sqrt{l(l-1)} & k=l-2\\ \frac{1}{2}(2l+1) & k=l\\ \frac{1}{2}\sqrt{(l+1)(l+2)} & k=l+2\\ 0 & \text{otherwise}\end{cases}\end{aligned} \tag{23}$$

where $x_0=\sqrt{2\mu(T)}$.
